# Supplementary material for: SMORE: Score Models for Offline Goal-Conditioned Reinforcement Learning
Source: arXiv:2311.02013 source file (2024-02-29)
Supplement: Supplementary file 1 [file appendix_scogo_suboptimality_bound2.tex]

\subsection{Suboptimality Bound for \scogo}
\label{sec:scogo_proof}

\scogoVperformance*
\begin{proof}

Let $y(s,a,g)=\gamma \sum_{s'} p(s'|s,a,g)S(s',g)-S(s,g)$. Starting with the action-free objective for \scogo:
\begin{align}
g(d,S)&=  (1-\gamma)\E{d_0(s,g)}{S(s,g)} \nonumber 
    +\E{s,a\sim \dmix}{y(s,a,g)}\nonumber\\
    &-(1-\beta) \E{s,a\sim d^S}{y(s,a,g)}-\f{\dmix}{\demix}
\end{align}

In the derivation for the final form of \scogo, we replace the inner maximization with its closed-form solution. To generate the closed form solution the following importance sampling step is performed:
\begin{align}
g'(d,S)&= (1-\gamma)\E{d_0(s,g)}{S(s,g)} \nonumber 
    +\E{s,a\sim \demix}{\frac{\dmix}{\demix}y(s,a,g)}\nonumber\\
    &-(1-\beta) \E{s,a\sim d^S}{y(s,a,g)}-\f{\dmix}{\demix}
\end{align}

Under our assumption that the set of visitations the pessimistic policy optimization procedure searches over is $d \in D_\eta$ 
\begin{equation}
    \abs{g(d,S) - g'(d,S)} \to  \abs{\E{\dmix}{ \mathcal{T}_0S(s, a, g)-S(s, g)} - \E{\demix}{\tfrac{\dmix}{\demix}\left( \mathcal{T}_0S(s, a, g)-S(s, g)\right)}}.
\end{equation}
For any visitation distribution $d \in D_\eta$, it holds that
\begin{align}
  & \abs{\E{\dmix}{( \mathcal{T}_0S(s, a, g)-S(s, g))}-\E{\demix}{\tfrac{\dmix}{{\demix}}( \mathcal{T}_0S(s, a, g)-S(s, g))}}\nonumber \\
 & \leq \E{ s,a,g \in \text{Support}(d) \backslash \text{Support}(d^{Q,O}_{mix})}{\abs{ \mathcal{T}_0S(s, a, g)-S(s, g)}} \le  \eta \max \abs{ \mathcal{T}_0S(s, a, g) -S(s, g)}
 \le \eta R_{\max},
\end{align}
\hs{Ahmed: This holds for 1 probability distribution. Union bound over all possible distributions}
With finite samples we use an empirical estimator for $g'(d,S)$ with the resulting estimator denoted by $\hat{g'}(d,S)$. Under the given assumption of a pessimistic policy search procedure which only searches for visitations(and corresponding policies) within $D_\eta$ that have $D_{KL}(\dmix \| \demix)\le \alpha$, we can bound weighted empirical loss for importance sampling~\citep{cortes2010learning} as follows: 

\begin{equation}
    \abs{g'(d,S)-\hat{g'}(d,S)} \le 2^{5/4}\sqrt{\alpha} \left(\frac{\text{Pdim}(\mathcal{R})\log(2Ne/\text{Pdim}(\mathcal{R}))+\log(4/\delta)}{N}\right)^{3/8} ~\forall d
\end{equation}
where $\text{Pdim}$ denotes the pseudo dimension or Pollard's dimension of the function class.

Combining both the results above we have our approximation error of the resulting objective that the value function is optimized with:

\begin{align}
    \abs{g(d,S)-\hat{g'}(d,S)} &=\abs{g(d,S)-g'(d,S)+g'(d,S)-\hat{g'}(d,S)}\\
    & \le \abs{g(d,S)-g'(d,S)} + \abs{g'(d,S)-\hat{g'}(d,S)}\\
    & \le \eta R_{\max} +  2^{5/4}\sqrt{\alpha} \left(\frac{\text{Pdim}(\mathcal{R})\log(2Ne/\text{Pdim}(\mathcal{R}))+\log(4/\delta)}{N}\right)^{3/8}
\end{align}
    
We will use $\epsilon_\texttt{ScoGo}$ to denote the approximation error upper bound $\eta R_{\max} +  2^{5/4}\sqrt{\alpha} \left(\frac{\text{Pdim}(\mathcal{R})\log(2Ne/\text{Pdim}(\mathcal{R}))+\log(4/\delta)}{N}\right)^{3/8}$.

\subsubsection{Performance Bound of the Learned Policy}
\label{app:perf_bound_recoil_v}

% In the offline setting, akin to pessimism principle in offline RL, we aim to return the closest-to-expert in-dataset policy. We will see that \texttt{ReCOIL}-V can naturally incorporate such pessimism using implicit maximization. Assuming that \texttt{ReCOIL} can enforce this constraint approximately (searches for a policy visitation within $D_\delta$), we derive its performance error. For ease of notation we denote the oracle objective which searches for visitations within $D$ in Eq.~\eqref{eq:recoil_objective_imitation} as $\min_V \max_d g(d,V)$ and the realistic objective which searches for visitations within $D_\delta$ in Eq.~\eqref{eq:recoil_objective_imitation} as $\min_V \max_d \hat{g}(d,V)$. Let the gap between these two objectives is given to be upper bounded by an approximation error denoted by $\epsilon_\text{approx}$. \qq{I think there shouldn't be $D$? only needs $D_\delta$}
 Recall that $\epsilon_\texttt{ScoGo}$ denotes the approximation error of the objective function in \scogo:
\begin{equation}
\label{eq:bounded_approx_error}
    \epsilon_\texttt{ScoGo} = \max_{d \in D_\eta} \abs{g(d,S)- \hat{g'}(d,S)}.
\end{equation}

Let $h(S) = \max_{d \in D_\eta} g(d,S)$ and $\hat{h}(S) = \max_{d \in D_\eta}  \hat{g}(d,S)$. It directly follows from Eq.~\eqref{eq:bounded_approx_error}
that 
\begin{equation}
\label{eq:abs_bound_h}
    |\hat{h}(S) - h(S)| \le 2\epsilon_\texttt{ScoGo}, \; \forall S.
\end{equation}
% We note that $\max_{d} g(d,S)$ (without the $d \in D_\eta$ constraint) is the standard \dualV form for imitation learning, but $h(S)$ here is defined as the same optimization under a constrained set $d \in D_\eta$.

% \paragraph{Step 1.} We first show that both $h$ and $\hat{h}$ are convex functions of $V$.
% Recall the definition of $\hat{h}(V)$:
% \begin{align}
% \hat{h}(V) = \min_V \max_d \beta(1-\gamma)\E{d_0(s)}{V(s)} + \E{s,a\sim \demix}{\frac{d^{R}_\text{mix}(s,a)}{\demix}(\gamma \mathcal{T}_0V(s, a)-V(s))} - \E{\demix}{f\left(\frac{\dmix}{\demix}\right)} \nonumber \\- (1-\beta) \E{d^R}{\gamma \mathcal{T}_0V(s, a)-V(s)}
% \end{align}
% which can be simplified using a closed form solution for inner maximization:
% \begin{align}
% \hat{h}(V) = \min_V  \beta(1-\gamma)\E{d_0(s)}{V(s)} + \E{s,a\sim \demix}{f^*_p(\gamma \mathcal{T}_0V(s, a)-V(s))} - (1-\beta) \E{d^R}{\gamma \mathcal{T}_0V(s, a)-V(s)}
% \end{align}
% The first and last term above are linear in $V$ and all that remains is to
% We also note that $h$ and $\hat{h}$ is  $\kappa$-strongly convex with  $\kappa$  given in Table~\ref{tab:strong_convexity}.

Let $\hat{S} = \argmin_S \hat{h}(S)$ and $ S^* = \argmin_S h(S) $. We are interested
in bounding the gap $h(\hat{S}) - h(S^*)$. It holds that
\begin{align}
        h(\hat{S}) - h(S^*) 
    & = h(\hat{S}) - \hat{h}(\hat{S}) + \hat{h}(\hat{S}) - h(S^*) \\
    & = h(\hat{S}) - \hat{h}(\hat{S}) + \hat{h}(\hat{S}) - \hat{h}(S^*) + \hat{h}(S^*) - h(S^*) \\
    & \leq 2\epsilon_\texttt{ScoGo} + 0 + 2\epsilon_\texttt{ScoGo} \\
    & = 4 \epsilon_\texttt{ScoGo},
\end{align}
where the inequality follows from Eq.~\eqref{eq:abs_bound_h} and the fact $\hat{S} = \argmin_S \hat{h}(S)$.

As a consequence, we have
\begin{align}
    4 \epsilon_\texttt{ScoGo}
& \geq h(\hat{S}) - h(S^*) \\
& \geq h(S^*) + (S^*-\hat{S})\nabla h(S^*) + \frac{\kappa}{2}\|S^*-\hat{S}\|^2_F - h(S^*) \\
& = \frac{\kappa}{2}\|S^*-\hat{S}\|^2_F,
\end{align}
where the second inequality comes from the fact that the function $h(S)$ is $\kappa$-strongly convex and
$\nabla h(V^*) = 0$. It directly follows
that
\begin{align}
    \|S^*-\hat{S}\|_\infty \leq \|S^*-\hat{S}\|_F \leq  2\sqrt{\tfrac{2}{\kappa} \epsilon_\texttt{ScoGo}}.
\end{align}

 Let $\pi^*_g$ be the policy that acts greedily with value function $S^*$, which is an optimal policy over all policies whose visitation distribution is within $D_\eta$. Since $d^*$ or the optimal policy visitation is a feasible visitation in $D_\eta$, $S^*$ represents the score for the optimal visitation.
 
 Let $\hat{\pi}_g$ denote the policy that acts greedily with value function $\hat{S}$, i.e., the output policy of \scogo. We then use the results in~\citet{singh1994upper} to bound the performance gap between $\pi^*_g$ and $\hat{\pi}_g$:
 \todoah{S is not a value function of the reward and $\pi_g$ is not the greedy policy with respect of S, I am not sure how the analysis works here.}
\begin{equation}
    J^{\pi^*_g} - J^{\hat{\pi}_g} \le \frac{4}{1-\gamma} \sqrt{\frac{2\epsilon_\texttt{ScoGo}}{\kappa}} \leq  \frac{4}{1-\gamma} \sqrt{\frac{2}{\kappa} \left(\eta R_{\max} +  2^{5/4}\sqrt{\alpha} \left(\frac{\text{Pdim}(\mathcal{R})\log(2Ne/\text{Pdim}(\mathcal{R}))+\log(4/\delta)}{N}\right)^{3/8}\right)}.
\end{equation}

This concludes the proof for Theorem~\ref{thm:scogoVperformance}. The first term is the irreducible error of missing coverage of optimal policy visitation in the offline dataset. The second term in the square root represents the finite sample error that goes to 0 as the number of samples N goes to infinity.
\end{proof}
