# Supplementary material for: SMORE: Score Models for Offline Goal-Conditioned Reinforcement Learning
Source: arXiv:2311.02013 source file (2024-02-29)
Supplement: Supplementary file 2 [file appendix_scogo_suboptimality_bound.tex]

\subsection{Suboptimality Bound for \scogo}
\label{sec:scogo_proof}

Let $y(s,a,g)=\gamma \sum_{s'} p(s'|s,a,g)S(s',g)-S(s,g)$. Starting with the action-free objective for \scogo:
\begin{align}
g(d,V)&= \min_{S(s,a,g)}  \max_{\dmix \ge0} (1-\gamma)\E{d_0(s,g)}{S(s,g)} \nonumber 
    +\E{s,a\sim \dmix}{y(s,a,g)}\nonumber\\
    &-(1-\beta) \E{s,a\sim d^S}{y(s,a,g)}-\f{\dmix}{\demix}
\end{align}

In the derivation for the final form of \scogo, we replace the inner maximization with its closed-form solution. To generate the closed form solution the following importance sampling step is performed:
\begin{align}
g'(d,V)&= \min_{S(s,g)}  \max_{\dmix \ge0} (1-\gamma)\E{d_0(s,g)}{S(s,g)} \nonumber 
    +\E{s,a\sim \demix}{\frac{\dmix}{\demix}y(s,a,g)}\nonumber\\
    &-(1-\beta) \E{s,a\sim d^S}{y(s,a,g)}-\f{\dmix}{\demix}
\end{align}

Under our assumption that the set of visitations the pessimistic policy optimization procedure searches over is $d \in D_\eta$ 
\begin{equation}
    \abs{g(d,V) - g'(d,V)} \to  \abs{\E{\dmix}{ \mathcal{T}_0V(s, a)-V(s)} - \E{\demix}{\tfrac{\dmix}{\demix}\left( \mathcal{T}_0V(s, a)-V(s)\right)}}.
\end{equation}
For any visitation distribution $d \in D_\eta$, it holds that
\begin{align}
  & \abs{\E{\dmix}{( \mathcal{T}_0V(s, a)-V(s))}-\E{\demix}{\tfrac{\dmix}{{\demix}}( \mathcal{T}_0V(s, a)-V(s))}}\nonumber \\
 & \leq \E{ s,a \in \text{Support}(d) \backslash \text{Support}(d^{Q,O}_{mix})}{\abs{ \mathcal{T}_0V(s, a)-V(s)}} \le \max \eta \abs{ \mathcal{T}_0V(s, a) - V(s)}
 \le \eta R_{\max},
\end{align}

With finite samples we use an empirical estimator for $g'(d,V)$ with resulting estimator denoted by $\hat{g'}(d,V)$. Using Hoeffdings inequality with importance-weighted empirical loss (with bounded coverage coefficient) we have that:
\begin{equation}
   \abs{g'(d,V)-\hat{g'}(d,V)} \le  M\sqrt{2\ln |\mathcal{V}|/N}
\end{equation}

Combining both the results above we have our approximation error of the resulting objective that the value function is optimized with:

\begin{align}
    \abs{g(d,V)-\hat{g'}(d,V)} &=\abs{g(d,V)-g'(d,V)+g'(d,V)-\hat{g'}(d,V)}\\
    & \le \abs{g(d,V)-g'(d,V)} + \abs{g'(d,V)-\hat{g'}(d,V)}\\
    & \le \eta R_{\max} +  M\sqrt{2\ln |\mathcal{V}|/N} 
\end{align}
    
We will use $\epsilon_\texttt{ScoGo}$ to denote the approximation error upper bound $\eta R_{\max} +  M\sqrt{2\ln |\mathcal{V}|/N}$.

\subsubsection{Performance Bound of the Learned Policy}
\label{app:perf_bound_recoil_v}

% In the offline setting, akin to pessimism principle in offline RL, we aim to return the closest-to-expert in-dataset policy. We will see that \texttt{ReCOIL}-V can naturally incorporate such pessimism using implicit maximization. Assuming that \texttt{ReCOIL} can enforce this constraint approximately (searches for a policy visitation within $D_\delta$), we derive its performance error. For ease of notation we denote the oracle objective which searches for visitations within $D$ in Eq.~\eqref{eq:recoil_objective_imitation} as $\min_V \max_d g(d,V)$ and the realistic objective which searches for visitations within $D_\delta$ in Eq.~\eqref{eq:recoil_objective_imitation} as $\min_V \max_d \hat{g}(d,V)$. Let the gap between these two objectives is given to be upper bounded by an approximation error denoted by $\epsilon_\text{approx}$. \qq{I think there shouldn't be $D$? only needs $D_\delta$}
\hs{Needs rewriting} Recall that $\epsilon_\texttt{ScoGo}$ denotes the approximation error of the objective function in \scogo:
\begin{equation}
\label{eq:bounded_approx_error}
    \epsilon_\texttt{ScoGo} = \max_{d \in D_\eta, V} \abs{g(d,V)- \lim_{\beta \to 1}\hat{g'}(d,V)}.
\end{equation}

Let $h(V) = \max_{d \in D_\delta} g(d,V)$ and $\hat{h}(V) = \max_{d \in D_\delta} \lim_{\beta \to 1} \hat{g}(d,V)$. It directly follows from Eq.~\eqref{eq:bounded_approx_error}
that 
\begin{equation}
\label{eq:abs_bound_h}
    |\hat{h}(V) - h(V)| \le 2\epsilon_\texttt{ReCOIL}, \; \forall V.
\end{equation}
We note that $\max_{d} g(d,V)$ (without the $d \in D_\delta$ constraint) is the standard \dualV form for imitation learning, but $h(V)$ here is defined as the same optimization under a constrained set $d \in D_\delta$.

% \paragraph{Step 1.} We first show that both $h$ and $\hat{h}$ are convex functions of $V$.
% Recall the definition of $\hat{h}(V)$:
% \begin{align}
% \hat{h}(V) = \min_V \max_d \beta(1-\gamma)\E{d_0(s)}{V(s)} + \E{s,a\sim \demix}{\frac{d^{R}_\text{mix}(s,a)}{\demix}(\gamma \mathcal{T}_0V(s, a)-V(s))} - \E{\demix}{f\left(\frac{\dmix}{\demix}\right)} \nonumber \\- (1-\beta) \E{d^R}{\gamma \mathcal{T}_0V(s, a)-V(s)}
% \end{align}
% which can be simplified using a closed form solution for inner maximization:
% \begin{align}
% \hat{h}(V) = \min_V  \beta(1-\gamma)\E{d_0(s)}{V(s)} + \E{s,a\sim \demix}{f^*_p(\gamma \mathcal{T}_0V(s, a)-V(s))} - (1-\beta) \E{d^R}{\gamma \mathcal{T}_0V(s, a)-V(s)}
% \end{align}
% The first and last term above are linear in $V$ and all that remains is to
% We also note that $h$ and $\hat{h}$ is  $\kappa$-strongly convex with  $\kappa$  given in Table~\ref{tab:strong_convexity}.

Let $\hat{V} = \argmin_V \hat{h}(V)$ and $ V^* = \argmin_V h(V) $. We are interested
in bounding the gap $h(\hat{V}) - h(V^*)$. It holds that
\begin{align}
        h(\hat{V}) - h(V^*) 
    & = h(\hat{V}) - \hat{h}(\hat{V}) + \hat{h}(\hat{V}) - h(V^*) \\
    & = h(\hat{V}) - \hat{h}(\hat{V}) + \hat{h}(\hat{V}) - \hat{h}(V^*) + \hat{h}(V^*) - h(V^*) \\
    & \leq 2\epsilon_\texttt{ScoGo} + 0 + 2\epsilon_\texttt{ScoGo} \\
    & = 4 \epsilon_\texttt{ScoGo},
\end{align}
where the inequality follows from Eq.~\eqref{eq:abs_bound_h} and the fact $\hat{V} = \argmin_V \hat{h}(V)$.

As a consequence, we have
\begin{align}
    4 \epsilon_\texttt{ScoGo}
& \geq h(\hat{V}) - h(V^*) \\
& \geq h(V^*) + (V^*-\hat{V})\nabla h(V^*) + \frac{\kappa}{2}\|V^*-\hat{V}\|^2_F - h(V^*) \\
& = \frac{\kappa}{2}\|V^*-\hat{V}\|^2_F,
\end{align}
where the second inequality comes from the fact that the function $h(V)$ is $\kappa$-strongly convex (Assumption 3) and
$\nabla h(V^*) = 0$. It directly follows
that
\begin{align}
    \|V^*-\hat{V}\|_\infty \leq \|V^*-\hat{V}\|_F \leq  2\sqrt{\tfrac{2}{\kappa} \epsilon_\texttt{ScoGo}}.
\end{align}

 Let $\pi^*_\delta$ be the policy that acts greedily with value function $V^*$, which is an optimal policy over all policies whose visitation distribution is within $D_\delta$. Let $\hat{\pi}$ denote the policy that acts greedily with value function $\hat{V}$, i.e., the output policy of \scogo. We then use the results in~\citet{singh1994upper} to bound the performance gap between $\pi^*_\delta$ and $\hat{\pi}$:
\begin{equation}
    J^{\pi^*_g} - J^{\hat{\pi}_g} \le \frac{4}{1-\gamma} \sqrt{\frac{2\epsilon_\texttt{ScoGo}}{\kappa}} \leq  \frac{4}{1-\gamma} \sqrt{\frac{2\delta R_{\max}}{\kappa}}.
\end{equation}

The above results demonstrate that \texttt{ReCOIL} is able to leverage suboptimal data with an approximate in-distribution policy improvement and results in a policy close to the best policy with visitation almost in-support of the dataset.
