# Supplementary material for: SMORE: Score Models for Offline Goal-Conditioned Reinforcement Learning
Source: arXiv:2311.02013 source file (2024-02-29)
Supplement: Supplementary file 3 [file appendix_scogo_suboptimality_bound3.tex]

\subsection{Suboptimality Bound for \scogo}
\label{sec:scogo_proof}

\scogoVperformance*
\begin{proof}

Let $y(s,a,g)=\gamma \sum_{s'} p(s'|s,a,g)S(s',g)-S(s,g)$. Starting with the action-free objective for \scogo:
\begin{align}
g(d,S)&=  (1-\gamma)\E{d_0(s,g)}{S(s,g)} \nonumber 
    +\E{s,a\sim \dmix}{y(s,a,g)}\nonumber\\
    &-(1-\beta) \E{s,a\sim d^S}{y(s,a,g)}-\f{\dmix}{\demix}
\end{align}

In the derivation for the final form of \scogo, we replace the inner maximization with its closed-form solution. To generate the closed form solution the following importance sampling step is performed:
\begin{align}
g'(d,S)&= (1-\gamma)\E{d_0(s,g)}{S(s,g)} \nonumber 
    +\E{s,a\sim \demix}{\frac{\dmix}{\demix}y(s,a,g)}\nonumber\\
    &-(1-\beta) \E{s,a\sim d^S}{y(s,a,g)}-\f{\dmix}{\demix}
\end{align}

Under our assumption of bounded coverage coefficient, $\forall d \in D_M$, $g'(d,S)=g(d,S)$

% Under our assumption that the set of visitations the pessimistic policy optimization procedure searches over is $d \in D_\eta$ 
% \begin{equation}
%     \abs{g(d,S) - g'(d,S)} \to  \abs{\E{\dmix}{ \mathcal{T}_0S(s, a, g)-S(s, g)} - \E{\demix}{\tfrac{\dmix}{\demix}\left( \mathcal{T}_0S(s, a, g)-S(s, g)\right)}}.
% \end{equation}
% For any visitation distribution $d \in D_\eta$, it holds that
% \begin{align}
%   & \abs{\E{\dmix}{( \mathcal{T}_0S(s, a, g)-S(s, g))}-\E{\demix}{\tfrac{\dmix}{{\demix}}( \mathcal{T}_0S(s, a, g)-S(s, g))}}\nonumber \\
%  & \leq \E{ s,a,g \in \text{Support}(d) \backslash \text{Support}(d^{Q,O}_{mix})}{\abs{ \mathcal{T}_0S(s, a, g)-S(s, g)}} \le  \eta \max \abs{ \mathcal{T}_0S(s, a, g) -S(s, g)}
%  \le \eta R_{\max},
% \end{align}
% \hs{Ahmed: This holds for 1 probability distribution. Union bound over all possible distributions}
% With finite samples we use an empirical estimator for $g'(d,S)$ with the resulting estimator denoted by $\hat{g'}(d,S)$. 

In practice we compute the supremum of function $g'(d,S)$ w.r.t $d$ by using empirical distributions for $d^O$ and $d^Q$. Under the given assumption of a policy search procedure which only searches for visitations(and corresponding policies) within $D_M$, we can bound weighted empirical loss with finite samples $N$ for importance sampling~\citep{cortes2010learning} as follows for any hypothesis $y\in\mathcal{R}$ and any distribution $d$ as follows with probability $1-\delta$:

\begin{equation}
     \abs{g'(d,S)-\hat{g'}(d,S)} \le M \sqrt{\frac{\log(2/\delta)}{2N}}
\end{equation}

Therefore, it holds with probability $1-\delta$ that $\forall d\in D_M, r \in \mathcal{R}$:

\begin{equation}
    \abs{g'(d,S)-\hat{g'}(d,S)} \le M \sqrt{\frac{\log((2|D_M||\mathcal{R}|)/\delta)}{2N}}
\end{equation}

We will use $\epsilon_\scogo$ to denote this approximation error upper bound

\subsubsection{Performance Bound of the Learned Policy}
\label{app:perf_bound_recoil_v}

 Recall that $\epsilon_\scogo$ denotes the approximation error of the objective function in \scogo:
\begin{equation}
\label{eq:bounded_approx_error}
    \epsilon_\scogo = \max_{d \in D_\eta} \abs{g(d,S)- \hat{g'}(d,S)}.
\end{equation}

Let $h(S) = \max_{d \in D_\eta} g(d,S)$ and $\hat{h}(S) = \max_{d \in D_\eta}  \hat{g}(d,S)$. It directly follows from Eq.~\eqref{eq:bounded_approx_error}
that 
\begin{equation}
\label{eq:abs_bound_h}
    |\hat{h}(S) - h(S)| \le 2\epsilon_\scogo, \; \forall S.
\end{equation}
% We note that $\max_{d} g(d,S)$ (without the $d \in D_\eta$ constraint) is the standard \dualV form for imitation learning, but $h(S)$ here is defined as the same optimization under a constrained set $d \in D_\eta$.

% \paragraph{Step 1.} We first show that both $h$ and $\hat{h}$ are convex functions of $V$.
% Recall the definition of $\hat{h}(V)$:
% \begin{align}
% \hat{h}(V) = \min_V \max_d \beta(1-\gamma)\E{d_0(s)}{V(s)} + \E{s,a\sim \demix}{\frac{d^{R}_\text{mix}(s,a)}{\demix}(\gamma \mathcal{T}_0V(s, a)-V(s))} - \E{\demix}{f\left(\frac{\dmix}{\demix}\right)} \nonumber \\- (1-\beta) \E{d^R}{\gamma \mathcal{T}_0V(s, a)-V(s)}
% \end{align}
% which can be simplified using a closed form solution for inner maximization:
% \begin{align}
% \hat{h}(V) = \min_V  \beta(1-\gamma)\E{d_0(s)}{V(s)} + \E{s,a\sim \demix}{f^*_p(\gamma \mathcal{T}_0V(s, a)-V(s))} - (1-\beta) \E{d^R}{\gamma \mathcal{T}_0V(s, a)-V(s)}
% \end{align}
% The first and last term above are linear in $V$ and all that remains is to
% We also note that $h$ and $\hat{h}$ is  $\kappa$-strongly convex with  $\kappa$  given in Table~\ref{tab:strong_convexity}.

Let $\hat{S} = \argmin_S \hat{h}(S)$ and $ S^* = \argmin_S h(S) $. We are interested
in bounding the gap $h(\hat{S}) - h(S^*)$. It holds that
\begin{align}
        h(\hat{S}) - h(S^*) 
    & = h(\hat{S}) - \hat{h}(\hat{S}) + \hat{h}(\hat{S}) - h(S^*) \\
    & = h(\hat{S}) - \hat{h}(\hat{S}) + \hat{h}(\hat{S}) - \hat{h}(S^*) + \hat{h}(S^*) - h(S^*) \\
    & \leq 2\epsilon_\scogo + 0 + 2\epsilon_\scogo \\
    & = 4 \epsilon_\scogo,
\end{align}
where the inequality follows from Eq.~\eqref{eq:abs_bound_h} and the fact $\hat{S} = \argmin_S \hat{h}(S)$.

As a consequence, we have
\begin{align}
    4 \epsilon_\scogo
& \geq h(\hat{S}) - h(S^*) \\
& \geq h(S^*) + (S^*-\hat{S})\nabla h(S^*) + \frac{\kappa}{2}\|S^*-\hat{S}\|^2_F - h(S^*) \\
& = \frac{\kappa}{2}\|S^*-\hat{S}\|^2_F,
\end{align}
where the second inequality comes from the fact that the function $h(S)$ is $\kappa$-strongly convex and
$\nabla h(V^*) = 0$. It directly follows
that
\begin{align}
    \|S^*-\hat{S}\|_\infty \leq \|S^*-\hat{S}\|_F \leq  2\sqrt{\tfrac{2}{\kappa} \epsilon_\scogo}.
\end{align}

 Let $\pi^*_g$ be the policy that acts greedily with value function $S^*$, which is an optimal policy over all policies whose visitation distribution is within $D_\eta$. Since $d^*$ or the optimal policy visitation is a feasible visitation in $D_\eta$, $S^*$ represents the score for the optimal visitation.

At convergence the following holds $\frac{\dmix}{\demix} = {{f^*_p}^'}(\gamma S(s'g)-S(s,g))$. 
 
 Let $\hat{\pi}_g$ denote the policy that acts greedily with value function $\hat{S}$, i.e., the output policy of \scogo. We then use the results in~\citet{singh1994upper} to bound the performance gap between $\pi^*_g$ and $\hat{\pi}_g$:
 \todoah{S is not a value function of the reward and $\pi_g$ is not the greedy policy with respect of S, I am not sure how the analysis works here.}
\begin{equation}
    J^{\pi^*_g} - J^{\hat{\pi}_g} \le \frac{4}{1-\gamma} \sqrt{\frac{2\epsilon_\texttt{ScoGo}}{\kappa}} \leq  \frac{4}{1-\gamma} \sqrt{\frac{2}{\kappa}  M \sqrt{\frac{\log((2|D_M||\mathcal{R}|)/\delta)}{2N}}}.
\end{equation}

This concludes the proof for Theorem~\ref{thm:scogoVperformance}. The first term is the irreducible error of missing coverage of optimal policy visitation in the offline dataset. The second term in the square root represents the finite sample error that goes to 0 as the number of samples N goes to infinity.
\end{proof}
